# Supplementary material for: Utilizing Longitudinal Chest X-Rays and Reports to Pre-Fill Radiology Reports
Source: arXiv:2306.08749 source file (2023-10-10)
Supplement: Supplementary file 1 [file 5_supplementary_material_v1.tex]

\section*{Supplementary Material}

\textbf{Hierarchical Memory-Driven Encoder} 

\noindent
\begin{figure}[!htbp]
  \centering
  \includegraphics[width=0.95\textwidth]{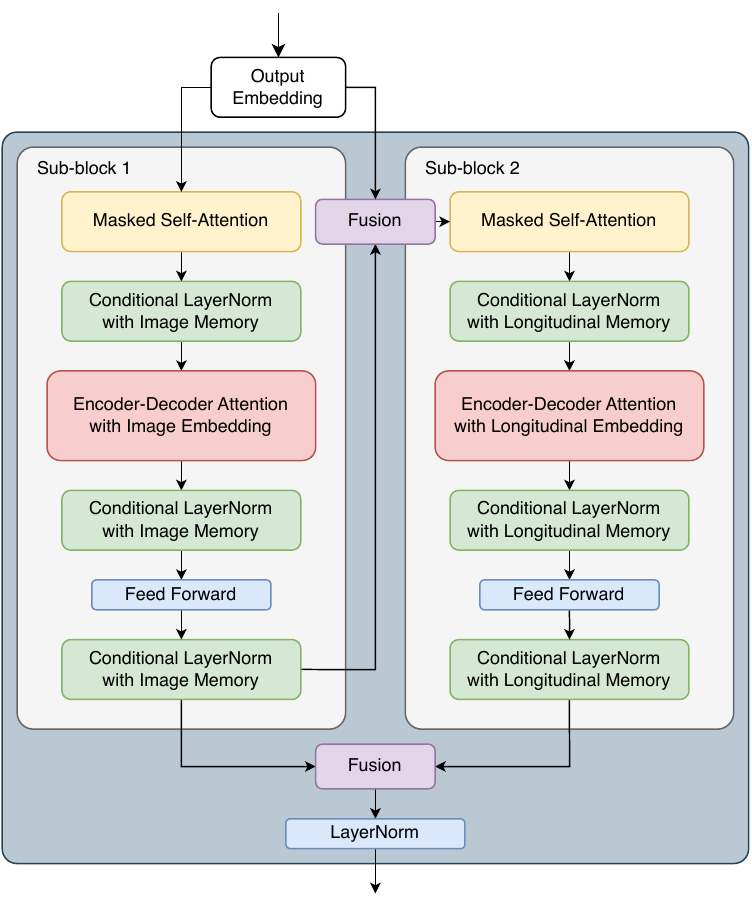}
  \caption{The sub-components of the hierarchical memory-driven decoder.}
  \label{decoder}
\end{figure}

\medskip
\noindent
\textbf{Implementation Details} 

\begin{table}[!htbp]\small 
    \centering
    \caption{Implementation Details}
    % \small % Adjust the font size here
    \begin{tabular}{>{\raggedright\arraybackslash}p{3cm}p{9cm}}
        \toprule
        \textbf{Component} & \textbf{Details} \\
        \midrule
        Pre-trained Model & ResNet-101 \\
        Feature Extraction & 2048 dimensions for each feature set from ImageNet \\
        Backbone Structure & Transformer with 3 layers, 8 attention heads, 512 hidden states dimensions \\
        Image Encoders & Same transformer-based encoder for current and previous images \\
        Text Encoder & Separate transformer encoder without shared parameters \\
        Initialization & Random initialization for transformers \\
        Relational Memory & 512 dimensions, 8 attention heads, 3 memory slots \\
        Loss Function & Cross-entropy loss at word level \\
        Training Epochs & 30 epochs \\
        Optimizer & ADAM optimizer \\
        Learning Rate & 5e-5 for visual extractor, 1e-4 for other parameters \\
        Learning Rate Decay & 0.8 per epoch \\
        \bottomrule
    \end{tabular}
\end{table}

\medskip
\noindent
\textbf{One more case}
\begin{figure}[h]
\centering
\includegraphics[width=0.95\textwidth]{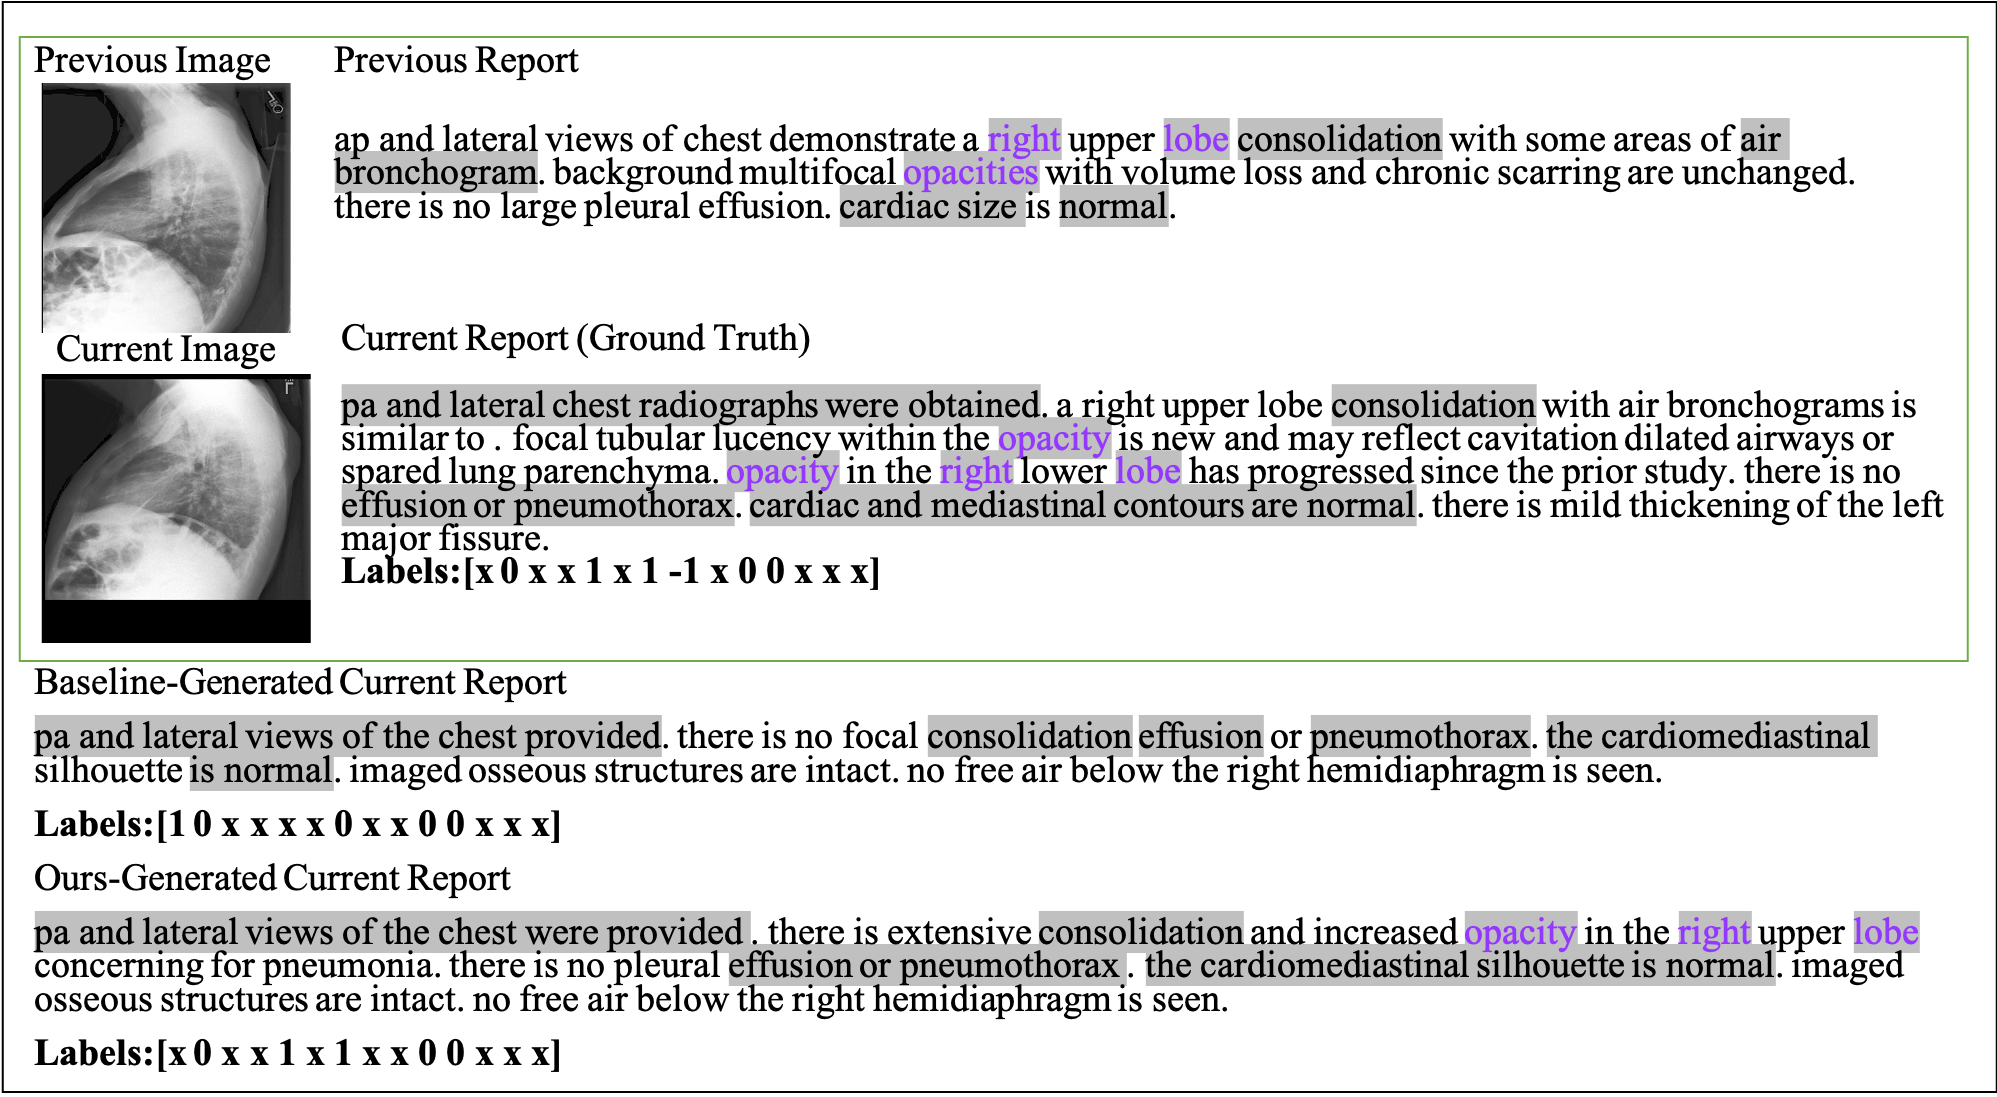}

% {figures/fig_case_study/case2.png}
\caption{An example of  pre-filled ``findings'' section of a report. }

\label{exap1}
\end{figure}
